# Supplementary material for: Exploring the Limits of ChatGPT in Software Security Applications
Source: arXiv:2312.05275 source file (2023-12-08)
Supplement: Supplementary file 1 [file appendix.tex]

% \appendix
